# Supplementary material for: Customizing ML Predictions for Online Algorithms
Source: arXiv:2205.08715 source file (2022-05-18)
Supplement: Supplementary file 1 [file appendix-kernelization.tex]

In this section, we want to illustrate how the margin based learner can incorporate {\em kernelization}.
where the main idea is to create a mapping of the data points in a (possibly infinite) dimension space where they become linearly separable.

\begin{definition}
A mapping function $\phi$ is said to be a $\nu$-bounded contraction iff for all $\norm{x}\leq 1$ it satisfies:
$$\norm{\phi(x_1) - \phi(x_2)} \geq \frac{1}{\nu} \cdot\norm{x_1-x_2}$$
\end{definition}

If the kernel $\phi(\cdot)$ satisfies the $\nu$-bounded contraction property then we can compose it with the Lipschitz property of the joint distribution $\mathbb{K}$ to show that:
$$\|y_1- y_2\| \leq L\nu \norm{\phi(x_1) - \phi(x_2)}$$. 
Indeed, popular kernels such as the polynomial kernel or the Gaussian kernel have the bounded contraction property. For instance, for the degree-2 polynomial kernel given by
$$\phi(x) = (1, x, x\otimes x)$$ satisfies $\nu$-bounded contraction for $\nu = 1$.%$\|\nabla \phi=\|\frac{d\phi}{dx}\| \geq \sqrt{2}\cdot e^{-\frac{1}{2\sigma^2}}$, for all $\abs{x}\le 1$ 

For clarity we repeat the performance result of Algorithm~\ref{algo: margin-based-pac} for kernels.
\begin{corollary*}
For a kernel function $\phi$ satisfying $\norm{\phi(x_1) - \phi(x_2)} \geq \frac{1}{\nu}\cdot\norm{x_1-x_2}$ for all $x_1, x_2$, assuming the data is linearly separable in kernel space, 
there exists a learning-to-rent algorithm that achieves a competitive ratio of $1+O\left(\frac{\sqrt{L\nu}}{n^{1/4}}\right)$ with $n$ samples
\end{corollary*}

Again the dimension independence of (Algorithm~\ref{algo: margin-based-pac}) allows us to exploit the kernelization to its fullest extent.
